# Supplementary material for: Federated Learning Meets Fairness and Differential Privacy
Source: arXiv:2108.09932 source file (2021-08-23)
Supplement: Supplementary file 1 [file appendix_GB.tex]

\appendix
\section{Generalization Bounds for FPFL}
We provide the lower bound on the expected cross-entropy loss. In our FL setting each agent $i \in \{1, \ldots, m\}$ owns data $(\mathcal{X}_i, \mathcal{A}_i, \mathcal{Y}_i) \sim \mathcal{D}_i$ i.e., it follows data distribution $\mathcal{D}_i$. We assume that the global data distribution is given by
$$ \mathcal{D} = \sum_{i=1}^m \frac{|\mathcal{X}_i|}{\mathbf{X}} \mathcal{D}_i$$

The objective function is to minimize the expected cross-entropy on the global data given by,

\begin{align*}
    \mathbb{E}_{((x,y) \sim \mathcal{D}}[l_{CE}(h^{\theta}, x, y)] &= \sum_{(x, y)} \mathcal{D} \cdot l_{CE}(h^{\theta}, x, y) \\
    &= \sum_{(x, y)} l_{CE}(h^{\theta}, x, y) \\
    &= \sum_{i=1}^m TBD
\end{align*}

\subsection{Phase 1}
In Phase 1 we minimize the loss $L_1$ given by Equation \ref{eqn::Phase1Loss}. We provide the generalization bounds for the first part of the loss given by $l_{CE}$, which is the cross entropy loss.

\begin{theorem}
For each agent $i$ having $m_i$ samples drawn from $\mathcal{D}_i$, for a fixed $\delta \in (0,1)$ with a probability at least $1 - \delta$
\begin{equation*}
        \begin{split}
 \mathbb{E}_{(x,y)\sim \mathcal{D}_i}[l_{CE}(f(x),y)] \leq \frac{1}{m_i} \sum_{j=1}^{m_i} l_{CE}&(f(x_j),y_j) + 
 2 \Omega_L  +  CL  \sqrt{\frac{\log (\frac{1}{\delta})}{m_i}}\\
        \end{split}{}
    \end{equation*}{}
\end{theorem}

\subsection{Phase 2}
In Phase 2 we minimize the loss $L_2$ given by Equation \ref{eqn::Phase2Loss}. 

\subsection{Combining Phase 1 and Phase 2
}
Given $\mathcal{Y} \in \{0,1\}$, i.e., binary classification problem. 
\begin{align}
    l_{CE}(h_{\phi}, y) &= - y \log (h_{\phi}) - (1-y) \log (1 - h_{\phi})\\
    l_{CE}(h_{\theta}, h_{\phi}) &= - h_{\phi} \log (h_{\theta}) - (1-h_{\phi}) \log (1 - h_{\theta}) 
    \label{eq:bce1}
\end{align}
We bound the loss $l_{CE}(h_{\theta}, y)$ in the following way,

\noindent First lets consider $y = 1$ and $h_{\theta}, h_{\phi} \in (0,1)$
\begin{align*}
    l_{CE}(h_{\theta}, y) &= -y \log(h_{\theta}) - (1-y)\log(1 - h_{\theta}) \\
    &= - \log(h_{\theta}) \quad \mbox{Since} \ y=1\\
    l_{CE}(h_{\phi}, y) &= - \log (h_{\phi}) \quad \mbox{Since} \ y=1 \\
    e^{- l_{CE}(h_{\phi}, y)} &= h_{\phi} \\
    l_{CE}(h_{\theta}, h_{\phi}) &= - e^{- l_{CE}(h_{\phi}, y)} \log (h_{\theta}) - (1-e^{- l_{CE}(h_{\phi}, y)}) \log (1 - h_{\theta}) \quad \mbox{Substitute in Equation \ref{eq:bce1}}\\
    l_{CE}(h_{\theta}, h_{\phi}) &\ge - e^{- l_{CE}(h_{\phi}, y)} \log (h_{\theta}) \quad \mbox{Since second term is always negative} \\
    l_{CE}(h_{\theta}, h_{\phi}) \cdot e^{l_{CE}(h_{\phi}, y)} & \ge - \log (h_{\theta})\\
    l_{CE}(h_{\theta}, y) &\leq l_{CE}(h_{\theta}, h_{\phi})  \cdot e^{l_{CE}(h_{\phi}, y)} \quad \mbox{By second equality}
\end{align*}

\noindent Consider the case when $y=0$
\begin{align*}
    l_{CE}(h_{\theta}, y) &= -y \log(h_{\theta}) - (1-y)\log(1 - h_{\theta}) \\
    &= - \log(1 - h_{\theta}) \quad \mbox{Since} \ y=0\\
    l_{CE}(h_{\phi}, y) &= - \log (1 - h_{\phi}) \quad \mbox{Since} \ y=0 \\
    e^{- l_{CE}(h_{\phi}, y)} &= 1-h_{\phi} \\
    l_{CE}(h_{\theta}, h_{\phi}) &= - (1-e^{- l_{CE}(h_{\phi}, y)}) \log (h_{\theta}) - e^{- l_{CE}(h_{\phi}, y)} \log (1 - h_{\theta}) \quad  \mbox{Substitute in Equation \ref{eq:bce1}} \\
    l_{CE}(h_{\theta}, h_{\phi}) &\ge - e^{- l_{CE}(h_{\phi}, y)} \log (1-h_{\theta}) \quad \mbox{Since first term is always negative} \\
    l_{CE}(h_{\theta}, h_{\phi}) \cdot e^{l_{CE}(h_{\phi}, y)} & \ge - \log (1 - h_{\theta})\\
    l_{CE}(h_{\theta}, y) &\leq l_{CE}(h_{\theta}, h_{\phi})  \cdot e^{l_{CE}(h_{\phi}, y)} \quad \mbox{By second equality}
\end{align*}

Hence we get the following relation,
\begin{equation}
    l_{CE}(h_{\theta}, y) \leq l_{CE}(h_{\theta}, h_{\phi})  \cdot e^{l_{CE}(h_{\phi}, y)} 
    \label{eq:rel}
\end{equation}
